# Supplementary material for: CURIE: An Iterative Querying Approach for Reasoning About Situations
Source: arXiv:2104.00814 source file (2021-04-05)
Supplement: Supplementary file 1 [file appendix.tex]

\clearpage
\appendix
\section{Appendix}
% \subsection{Polarity Words}

% \paragraph{Increasing words} \textit{helps, more, higher, increase, increases, stronger, faster, greater, longer, larger, helping}
% \paragraph{Decreasing words} \textit{hurts, less, lower, decrease, decreases, weaker, slower, smaller, hurting, softer, fewer}

\subsection{Hyperparameters}
\label{subsec:appendix_hyperparam}

\paragraph{Seq-to-Seq:} We use 2 layers of LSTM encoder and decoder with a hidden size of 500, word embedding size of 300. The encoder is bidirectional. We use Glove embedding of 300 dimensions.

\paragraph{\ours:}
\ours fine-tunes  \We use Adam~\cite{kingma2014adam} for optimization with a learning rate of $5e-05$.
All the dropouts~\cite{srivastava2014dropout} were set to 0.1
We found the best hyperparameter settings by searching the space using the following hyperparameters: 
    weight decay = \{ 0.1, 0.01, 0.05 \}, 
    embedding dropout = \{0.1, 0.2, 0.3 \}, 
    learning rate = \{1e-05, 2e-05, 5e-05, 1e-06\}
All experiments were done on a single Nvidia GeForce RTX 2080 Ti.
